# Supplementary material for: SVFusion: A CPU-GPU Co-Processing Architecture for Large-Scale Real-Time Vector Search
Source: arXiv:2601.08528 source file (2026-01-13)
Supplement: Supplementary file 1 [file appendix.tex]

\appendix

\section{Additional Exeperimental Results}
\label{appendix:exp-result}

\begin{figure*}[t] 
\centering
  \includegraphics[width=0.92\linewidth]{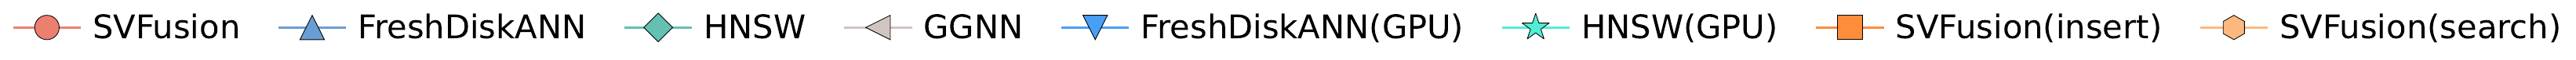}
  
  \begin{minipage}[t]{\textwidth}    
    \begin{minipage}[c]{0.035\textwidth}
      \raggedleft
      \rotatebox{90}{\small\parbox{2.5cm}{\centering Wikipedia-\\SlidingWindow}}
    \end{minipage}%
    \hspace{0.4em} 
    \begin{minipage}[c]{0.95\textwidth}
      \includegraphics[width=\linewidth]{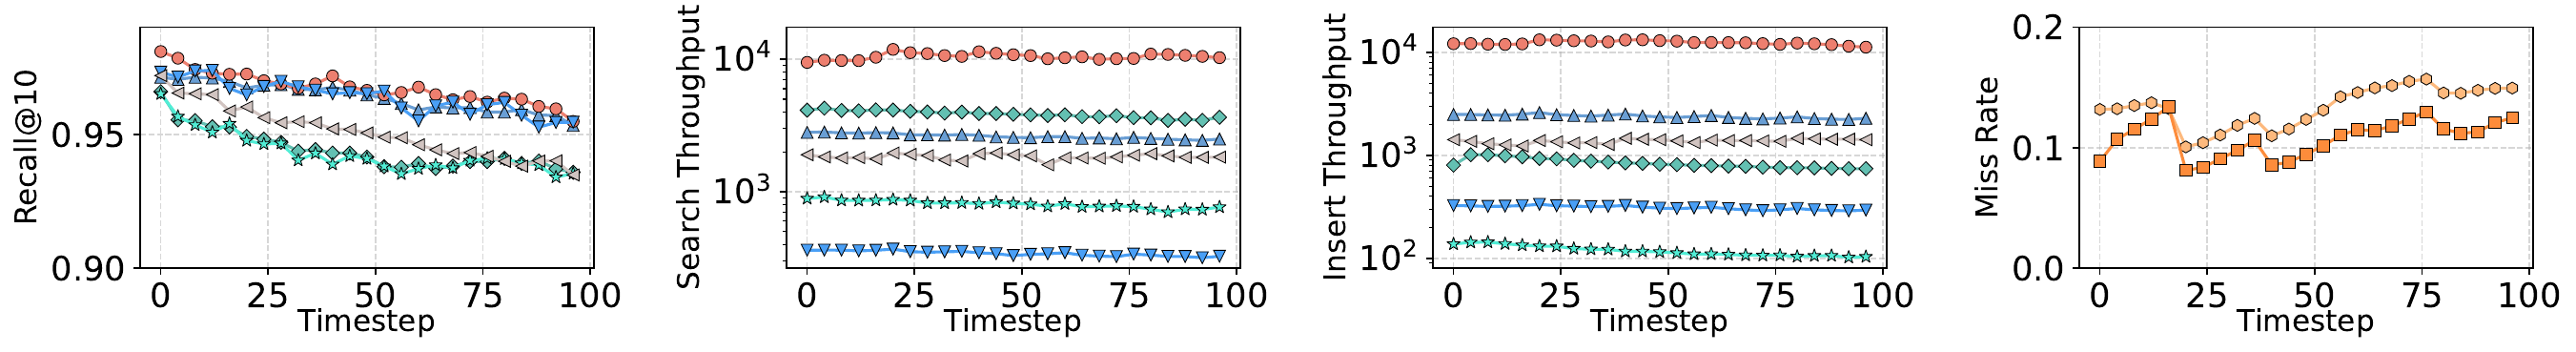}
    \end{minipage}
  \end{minipage}
  \vspace{-1em}
  
  \begin{minipage}[t]{\textwidth}     
    \begin{minipage}[c]{0.035\textwidth}
      \raggedleft
      \rotatebox{90}{\small\parbox{2.5cm}{\centering MSMARCO-\\SlidingWindow}}
    \end{minipage}%
    \hspace{0.6em}%  
    \begin{minipage}[c]{0.95\textwidth}
      \includegraphics[width=\linewidth]{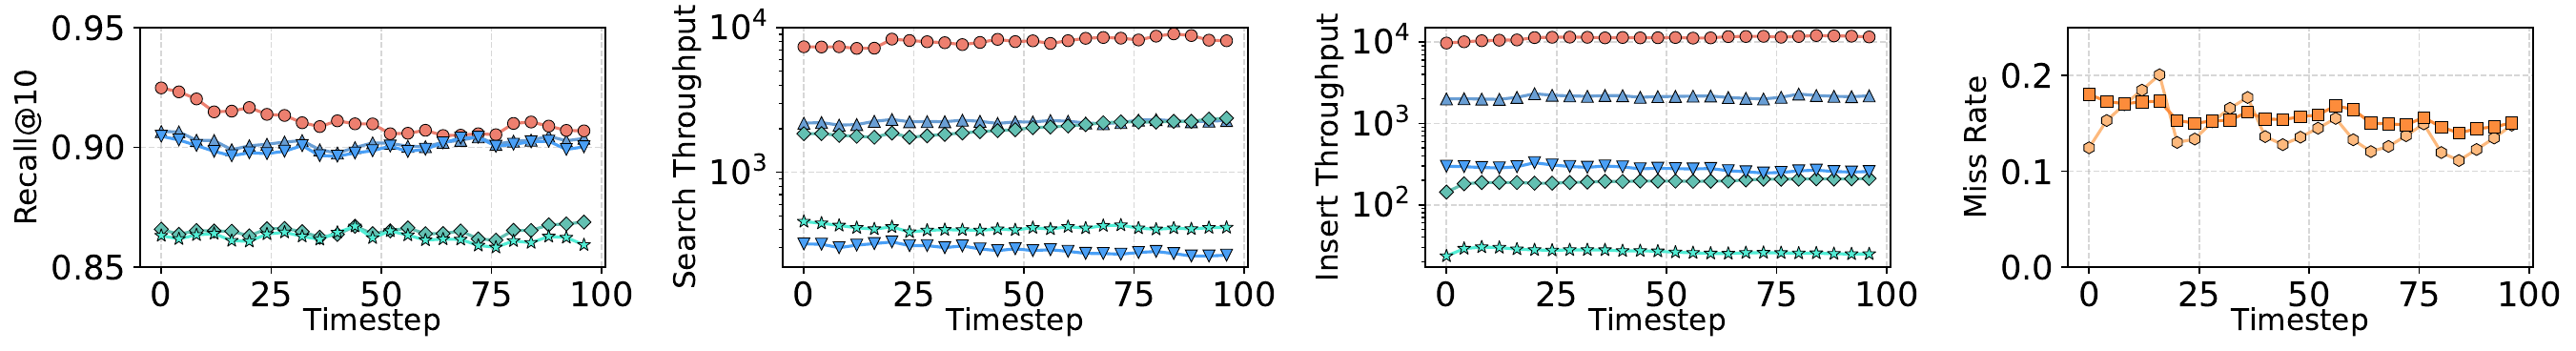}
    \end{minipage}
  \end{minipage}
  \vspace{-1em}
  
  \begin{minipage}[t]{\textwidth}      
    \begin{minipage}[c]{0.035\textwidth}
      \raggedleft
      \rotatebox{90}{\small\parbox{2.5cm}{\centering Wikipedia-\\Expiration}}
    \end{minipage}%
    \hspace{0.6em}% 
    \begin{minipage}[c]{0.95\textwidth}
      \includegraphics[width=\linewidth]{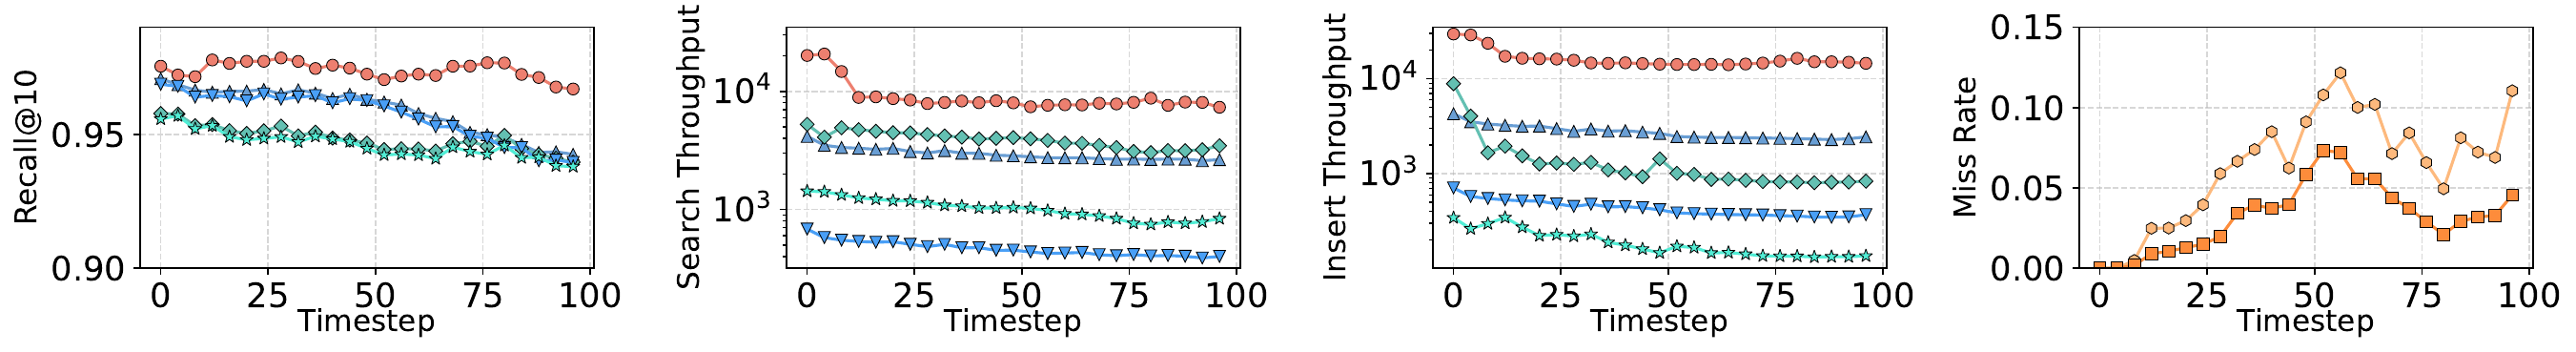}
    \end{minipage}
  \end{minipage}
  \vspace{-1em}
  
  \begin{minipage}[t]{\textwidth}      
    \begin{minipage}[c]{0.035\textwidth}
      \raggedleft
      \rotatebox{90}{\small\parbox{2.5cm}{\centering MSMARCO-\\Expiration}}
    \end{minipage}%
    \hspace{0.6em}%  
    \begin{minipage}[c]{0.95\textwidth}
      \includegraphics[width=\linewidth]{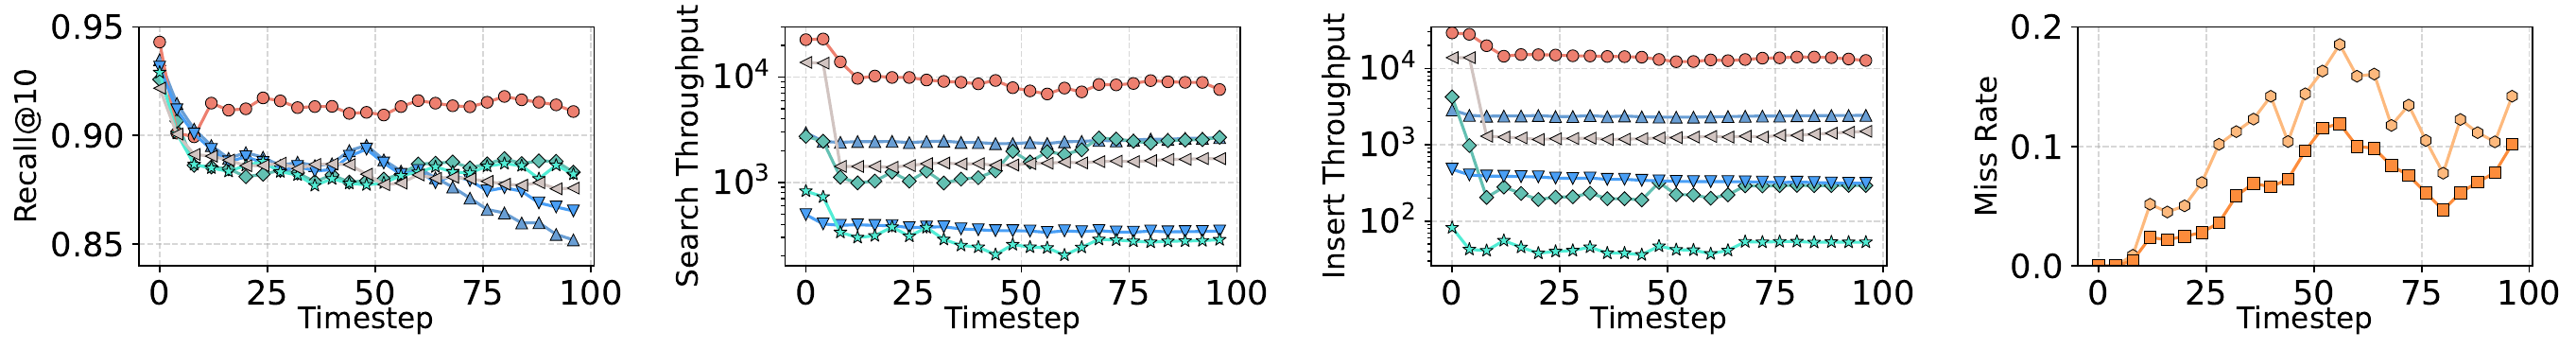}
    \end{minipage}
  \end{minipage}
  \vspace{-1em}

  \begin{minipage}[t]{\textwidth}      
    \begin{minipage}[c]{0.035\textwidth}
      \raggedleft
      \rotatebox{90}{\small\parbox{2.5cm}{\centering MSTuring-\\Clustered}}
    \end{minipage}%
    \hspace{0.6em}%  
    \begin{minipage}[c]{0.95\textwidth}
      \includegraphics[width=\linewidth]{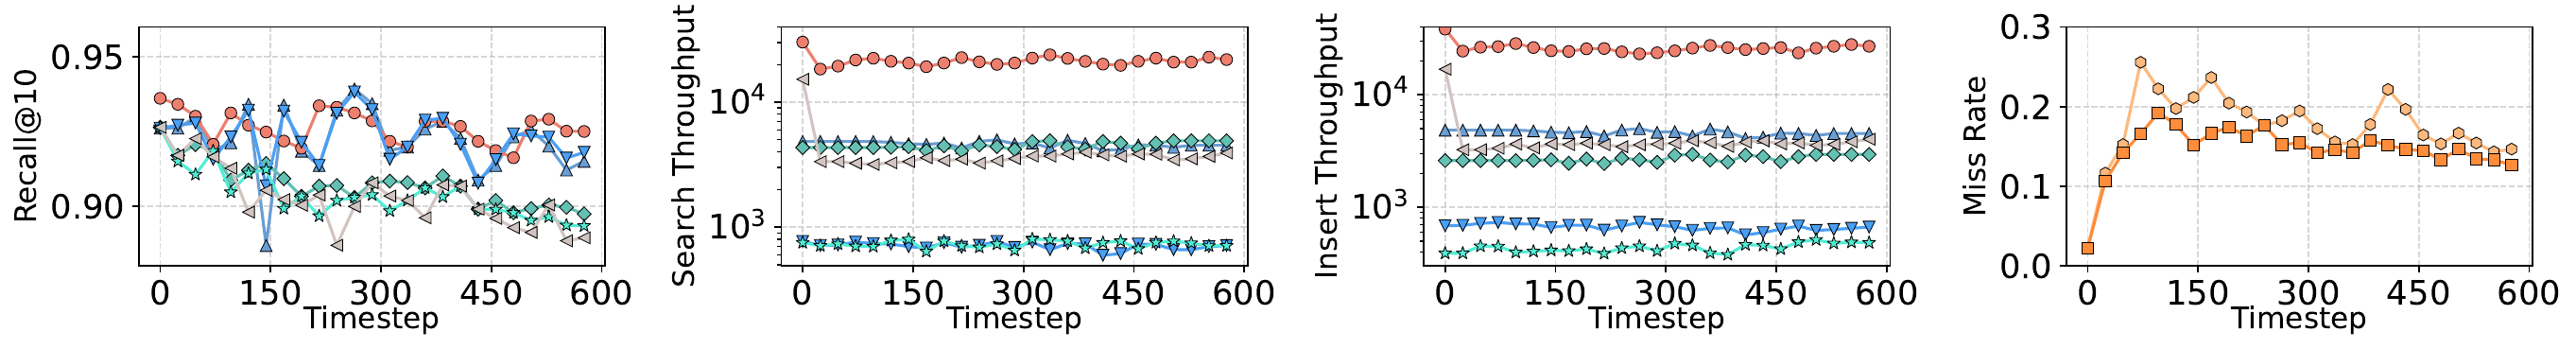}
    \end{minipage}
  \end{minipage}
  \vspace{-1em}

  \begin{minipage}[t]{\textwidth}      
    \begin{minipage}[c]{0.035\textwidth}
      \raggedleft
      \rotatebox{90}{\small\parbox{2.5cm}{\centering MSTuring-\\IH}}
    \end{minipage}%
    \hspace{0.6em}%  
    \begin{minipage}[c]{0.95\textwidth}
      \includegraphics[width=\linewidth]{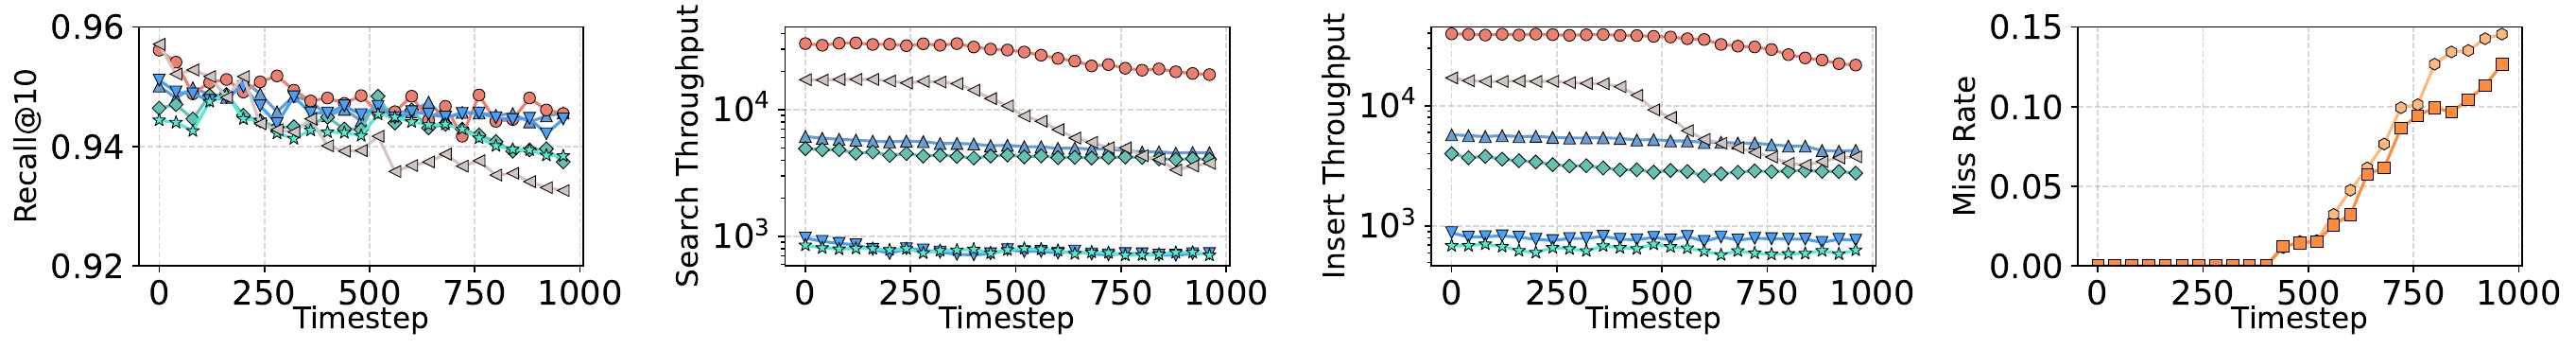}
    \end{minipage}
  \end{minipage}
  \vspace{-1em}

  \begin{minipage}[t]{\textwidth}      
    \begin{minipage}[c]{0.035\textwidth}
      \raggedleft
      \rotatebox{90}{\small\parbox{2.5cm}{\centering  Text2Image-\\Clustered}}
    \end{minipage}%
    \hspace{0.6em}%  
    \begin{minipage}[c]{0.95\textwidth}
      \includegraphics[width=\linewidth]{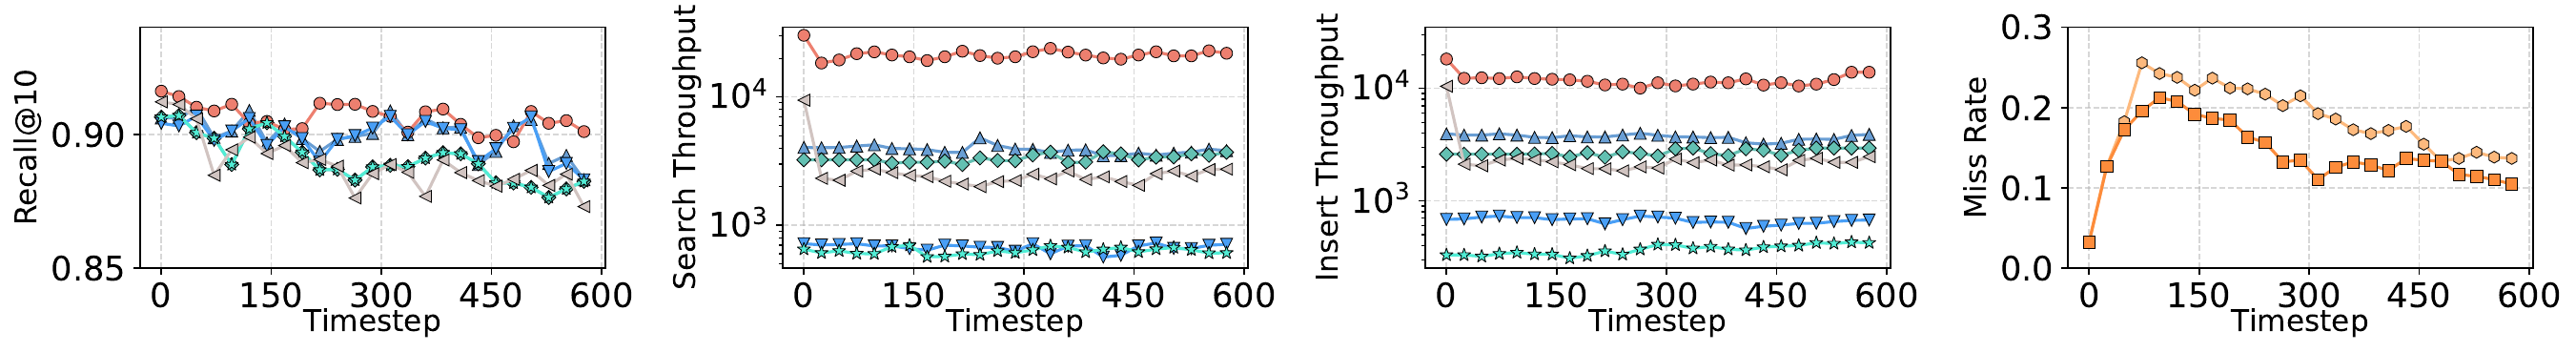}
    \end{minipage}
  \end{minipage}
  \vspace{-1em}
  
  \caption{\changeone{Comparison of recall, search throughput, insert throughput, and miss rate for seven various workloads.}}
  \label{fig:full_sanns_performance}
\vspace{-1em}
\end{figure*}

\textbf{Overall Performance}: Figure~\ref{fig:full_sanns_performance}
provides a comprehensive evaluation across all datasets and seven representative workloads, comparing recall, search throughput, insertion throughput, and cache miss rate. SVFusion consistently achieves high recall and maintains superior search and insert throughput across diverse workload patterns, including read-intensive, update-heavy, and mixed scenarios. The low and stable miss rate further demonstrates the effectiveness of our adaptive caching and coordination mechanisms in sustaining balanced performance under varying access dynamics.

\textbf{Deletion.} 
As shown in Table~\ref{tab:performance}, the lazy deletion time (tombstone marking) is comparable across all methods.
For graph repair efficiency, SVFusion significantly outperforms FreshDiskANN through our localized topology-aware repair strategy. Instead of relying on costly periodic graph reconstructions, SVFusion incrementally addresses connectivity issues.
This continuous maintenance prevents structural degradation while reducing both the complexity and frequency of consolidation, resulting in faster deletion processing.

\begin{table}[H]
  \centering
  \caption{Comparison of recall and running time (in seconds).}
  \label{tab:performance}
  \vspace{-1em}
  \footnotesize          
  \resizebox{\columnwidth}{!}{%
    \begin{tabular}{p{1.1cm}|l|c|c|c|p{0.6cm}p{0.6cm}}
      \toprule
      \multirow{2}{*}{\textbf{Workload}} & \multirow{2}{*}{\textbf{Method}} & \multirow{2}{*}{\textbf{Recall@10}} & \multirow{2}{*}{\textbf{Search}} & \multirow{2}{*}{\textbf{Insert}} & \multicolumn{2}{c}{\textbf{Delete}} \\
      \cmidrule{6-7}
      & & & & & \textbf{Mark} & \textbf{Repair} \\
      \midrule
      \multirow{3}{*}{\begin{tabular}[c]{@{}l@{}}Wikipedia\\-SW\end{tabular}}
        & FreshDiskANN & 96.38 & 98  & 6291  & 11 & 14795 \\
        & HNSW         & 94.41 & 55  & 18026 & 84 & -- \\
        & SVFusion     & \textbf{96.74} & \textbf{29} & \textbf{895} & \textbf{8} & \textbf{1207} \\
      \midrule
      \multirow{3}{*}{\begin{tabular}[c]{@{}l@{}}MSMARCO\\-SW\end{tabular}}
        & FreshDiskANN & 90.21 & 215 & 7058  & 16 & 18214 \\
        & HNSW         & 86.49 & 162 & 77666 & 86 & --  \\
        & SVFusion     & \textbf{91.12} & \textbf{56}  & \textbf{1336}  & \textbf{11} & \textbf{862} \\
      \midrule
      \multirow{3}{*}{\begin{tabular}[c]{@{}l@{}}Wikipedia\\-Exp\end{tabular}}
        & FreshDiskANN & 95.89 & 172 & 11142 & \textbf{21} & 2023 \\
        & HNSW         & 94.71 & 88  & 27537 & 149 & -- \\
        & SVFusion     & \textbf{97.39} & \textbf{58}  & \textbf{1891}  & 24 & \textbf{1082} \\
      \midrule
      \multirow{3}{*}{\begin{tabular}[c]{@{}l@{}}MSMARCO\\-Exp\end{tabular}}
        & FreshDiskANN & 88.39 & 379 & 12572 & 27 & 2463 \\
        & HNSW         & 88.38 & 392 & 117274 & 152 & -- \\
        & SVFusion     & \textbf{91.39} & \textbf{102} & \textbf{2065}  & \textbf{24} & \textbf{752} \\
      \midrule
      \multirow{3}{*}{\begin{tabular}[c]{@{}l@{}}MSTuring-\\Clustered\end{tabular}}
        & FreshDiskANN & 92.19 & 845 & 19122 & 41 & 21165 \\
        & HNSW         & 90.75 & 859 & 94776 & 188 & -- \\
        & SVFusion     & \textbf{92.74} & \textbf{167} & \textbf{3234} & \textbf{29} & \textbf{2183} \\
      \bottomrule
    \end{tabular}%
  }
\end{table}
